# Supplementary material for: Electrical conductivity of nanorod-based transparent electrodes: Comparison of mean-field approaches
Source: arXiv:2110.04455 source file (2021-10-09)
Supplement: Supplementary file 1 [file Tarasevich2021MFASupplement.pdf]

# Supplemental Material. Electrical conductivity of nanorod-based transparent electrodes: Comparison of mean-field approaches

Yuri Yu. Tarasevich,[1,*] Andrei V. Eserkepov,[1,†] and Irina V. Vodolazskaya[1,‡]

[1] *Laboratory of Mathematical Modeling, Astrakhan State University, Astrakhan 414056, Russia*

Figure S1 demonstrates the current distribution in a conductive wire for different variants of the mean-field approach. The reference wire (darker) is intersected by several other wires (lighter). Intersections (junctions) are highlighted. In the continuous variants of the mean-field approach, the junctions are "smeared" over the reference wire.

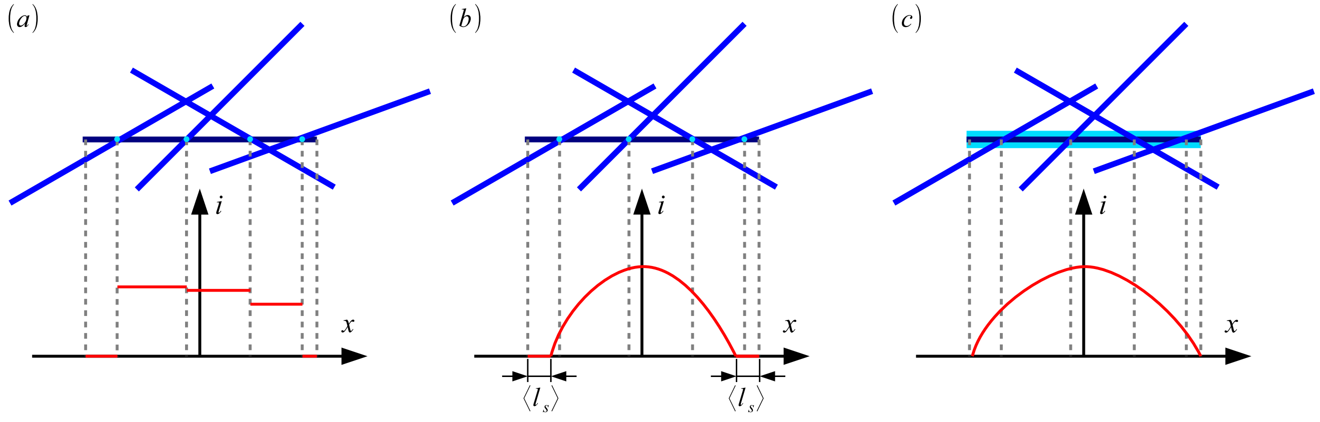


FIG. S1. Current distribution in different variants of the mean-field approach. (a) discrete, (b) hybrid, $\langle l_s \rangle$ is the mean segment length averaged over the entire system, (c) continuous.

Figure S2 demonstrates the dependencies of the electrical conductivity on the number density of the conductive wires for the wire resistance-dominated case and for the case when both resistances are equal. Different system sizes are used for comparison. No finite-size effect can be observed within the limits of computational accuracy.

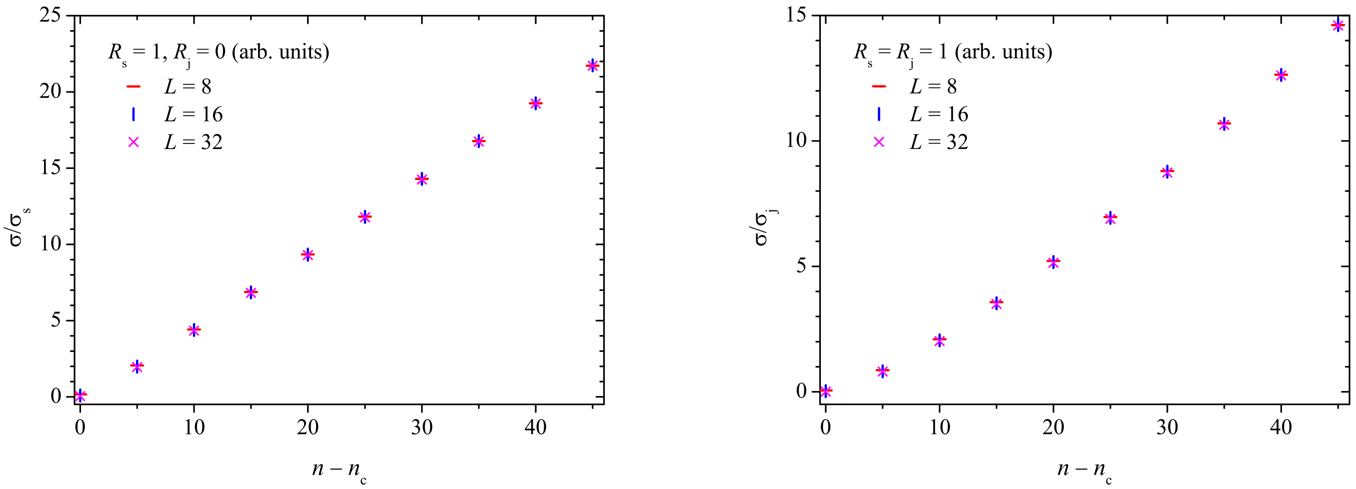


FIG. S2. Electrical conductivity against the number density of the conductive wires for the wire resistance-dominated case and for the case when both resistances are equal.

* Corresponding author: tarasevich@asu.edu.ru
† dantealigjery49@gmail.com
‡ vodolazskaya_agu@mail.ru

Figure S3 presents the distribution of the electrical currents in segments of the wires. Dots correspond to the currents in the segments against the position of the segment center relative to the wire center. The solid curve corresponds to the mean value of the electrical current.

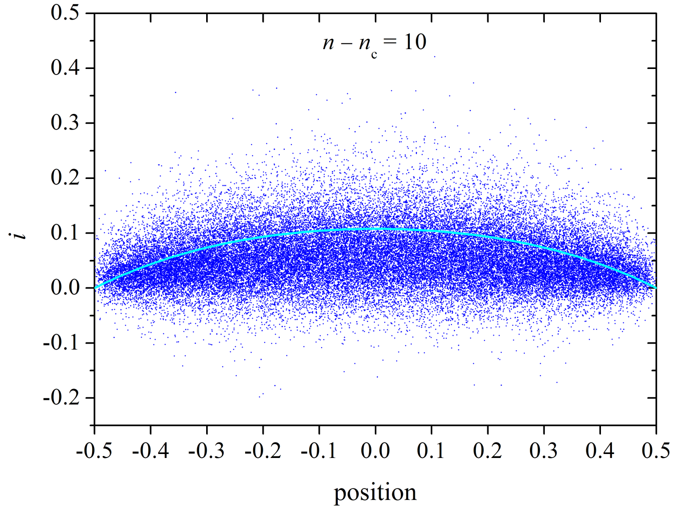


FIG. S3. Distribution of the electrical currents in the segments of wires. Dots correspond to the currents in segments against the position of the segment center relative to the wire center. Solid curve corresponds to the mean value of the electrical current.

Figure S4 demonstrates the dependencies of the electrical potential on the position of the junctions, for different ratios between the wire resistance and junction resistance and for different values of the number density of the conductive wires.

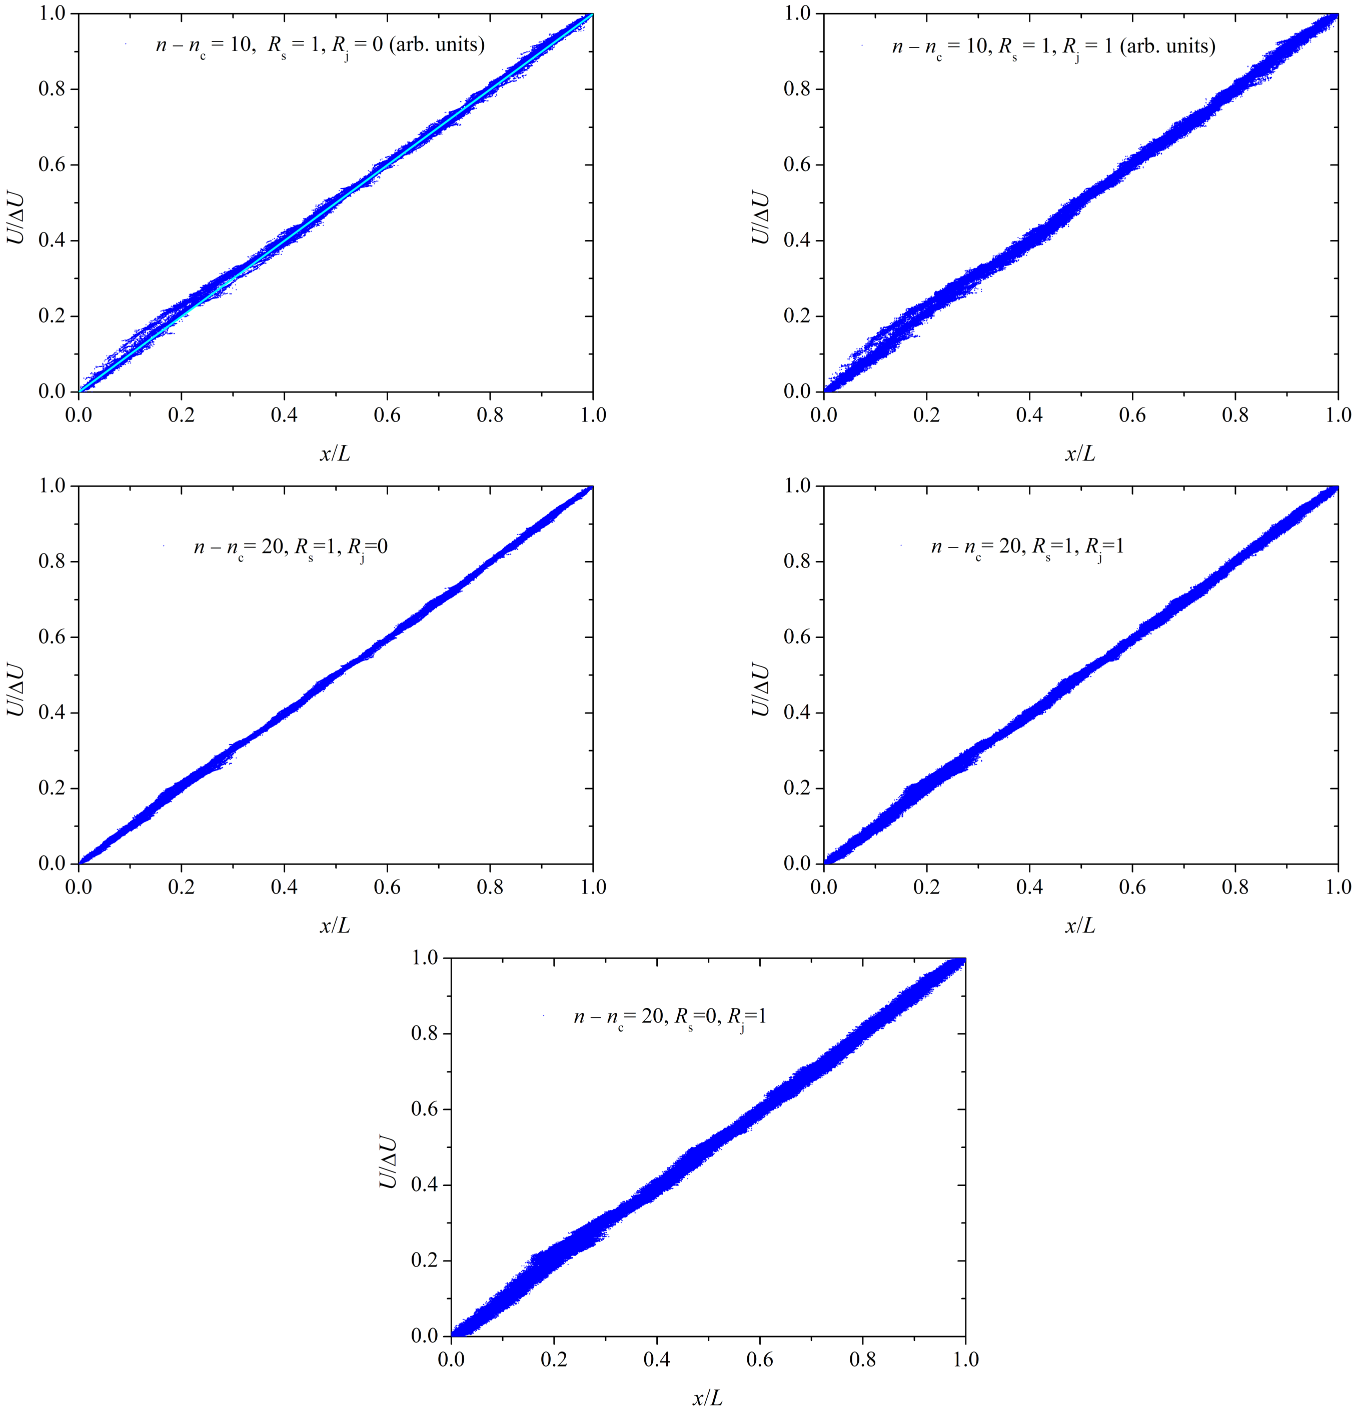


FIG. S4. Examples of the normalized potential, $U/\Delta U$, of each junction of the network plotted against its normalized position, $x/L$. The potential difference, $\Delta U$, is applied along the $x$-axis.
